# Supplementary material for: Effective Hamiltonians for the study of real metals using quantum chemical theories
Source: arXiv:2103.06318 source file (2021-03-10)
Supplement: Supplementary file 1 [file SI.pdf]

# Supporting Information for: Effective Hamiltonians for the study of real metals using quantum chemical theories

Tina N. Mihm[(a),(b)], Tobias Schäfer[(c)], Sai Kumar Ramadugu[(a),(b)], Andreas Grüneis[(c)], and James J. Shepherd[(a),(b)*]

[(a)] *Department of Chemistry, University of Iowa*

[(b)] *University of Iowa Informatics Initiative, University of Iowa*

[(c)] *Institute for Theoretical Physics, TU Wien, Wiedner Hauptstraße 8-10/136, 1040 Vienna, Austria*

## APPLICATION OF SFTA TO A METAL, AN INSULATOR, AND A SEMICONDUCTOR

In Fig. 1, box and whisker plots are used to show the results of using the transition structure factor from the selected twist angle to calculate the energy (sfTA) for a Na supercell containing 32 atoms it the body-centered phase. The distribution is drawn from 100 MP2 and 100 CCSD calculations with the average (mean) and quartiles shown. All points have their differences taken with the Γ-point i.e. this is a graph of Γ-point corrections. This allows us to compare the energies between the systems on a similar footing. It is important to note here that for some of the calculations, the Γ-point does not occur within the range of the 100 twist angles even when we include a small non-zero offset. The sfTA energy is shown to compare well with to the TA energy, with a difference between the TA- and sfTA-CCSD values of 3(1) meV/el and 1(2) meV/el for CCSD and MP2 respectively.

Also in Fig. 1, energy comparisons are made between sfTA and TA for other systems. Specifically, carbon (diamond lattice) and silicon (diamond lattice) are also included with both using an 8 atom supercells.This number of atoms ensures that all systems contain the same number of valence electrons (32). These are representative large-gap (insulating) to low-gap (metallic) systems. In general, for all three systems, the accuracy of sfTA continues to be comparable with twist averaging. Looking from left to right, we can see some trends as the band gap decreases. In particular, there is an increase in the width of the distribution of possible energies, although for Na this is also possibly attributable to there being more atoms. We also see the CCSD and MP2 energy distributions vary in how similar they are to each other. Although MP2 in general is well known to diverge into the TDL, it is not known whether the twist-averaged correction (with the Γ-point energy removed) also diverges. Overall, this diagram shows that sfTA can be applied to a variety of systems.

---

* james-shepherd@uiowa.edu

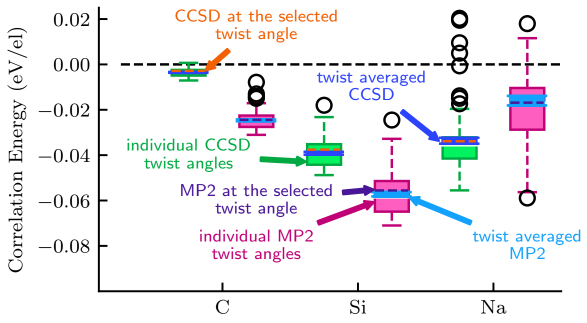


Figure 1. The sfTA-CCSD correlation energy for three systems with different band gaps are shown in comparison to both the TA energy and distribution of energies for all twist angles for CCSD and MP2. Energies are plotted as differences to the Γ-point. As can be seen in the graph, the three different systems all have comparable results between TA and sfTA. The silicon, sodium and carbon structure information was obtained from well known experimental lattice constants.
